# Supplementary material for: Verification of Neural Network Control Policy Under Persistent Adversarial Perturbation
Source: arXiv:1908.06353 source file (2019-08-18)
Supplement: Supplementary file 1 [file _App_additional_result.tex]

\section*{Appendix C: additional experiment result and discussion}

\textcolor{red}{TODO: need to rewrite this section as well.}

Here we provide some additional experiment results. The first neural network demonstrated in this section has an identical architecture to the one shown in Section \ref{sec:experiment} -- it is a $3$-layer neural network with $16$ neurons in each layer. The only difference is that this neural network is trained by behavior cloning of a LQR policy. The trained neural network policy is more linear around the equilibrium. Thus our certification method, which is based on linear robust control theory, is tighter. Table \ref{tab:add} shows our simulation result on this network model. If we compare Table \ref{tab:add} with Table \ref{tab:attack-L1}, we can see that the gap between the attack and the certified robustness decrease significantly. However, we also notice that the gap between our method (Algorithm \ref{alg:lin}) and the Lipschitz-based method becomes negligible. Therefore, our method offers less additional value on this network. For the network demonstrated in Section \ref{sec:experiment}, the neural network is highly nonlinear near the equilibrium point. In that case, Algorithm \ref{alg:lin} gives a significant advantage over the traditional Lipschitz-based method. 

\begin{table}[h!]
\centering
\caption{Additional comparison between the minimal attack distance and the certified robustness. This neural network is trained by behavior cloning of a LQR policy.}
\begin{adjustbox}{max width=1\textwidth}
    \begin{tabular}{c|c|c|c|cccc}
    \hline
    attack node & attack & Algo \ref{alg:lin} (Thm \ref{thm:LTI}) & Lipschitz-based & $\bar{x_1}$ & $\bar{x_2}$ & $\bar{x_3}$ & $\bar{x_4}$ \\
    \hline
      $u$ & 0.74219	& 0.34873	& 0.34873	& 0.39997	& 0.34454	& 2.32893	& 6.87542 \\
    $x_1$ & 0.83984	& 0.26523	& 0.26523	& 0.27679	& 0.23844	& 1.61170	& 4.75796\\
    $x_2$ & 0.34180	& 0.14482	& 0.14482	& 0.35430	& 0.30521	& 2.06306	& 6.09054\\
    $x_3$ & 1.39648	& 0.63789	& 0.63789	& 0.39066	& 0.33653	& 2.27474	& 6.71543 \\
    $x_4$ & 5.46875	& 2.38867	& 2.38867	& 0.37491	& 0.32296	& 2.18302	& 6.44465 \\
    \hline
    \end{tabular}%
    \end{adjustbox}
  \label{tab:add}%
\end{table}%

The second neural network is even more nonlinear than the one demonstrated in Section \ref{sec:experiment}. Table \ref{tab:add2} shows the result for a $3$-layer neural network with $32$ neurons at each layer. This network is more nonlinear near the equilibrium, and thus the gap between the minimal attack and the certified robustness become larger. Nevertheless, we also note that our certified robustness gives a significant advantage over the traditional Lipschitz-based method, with $16$ times improvement in average. 
%the neural network is highly nonlinear near the equilibrium point. In that case, Algorithm \ref{alg:lin} gives a significant advantage over the traditional Lipschitz-based method. 

\begin{table}[h!]
\centering
\caption{Additional comparison between the minimal attack distance and the certified robustness. This neural network has $3$ layers with $32$ neurons at each layer.}
\begin{adjustbox}{max width=1\textwidth}
    \begin{tabular}{c|c|c|c|cccc}
    \hline
    attack node & attack & Algo \ref{alg:lin} (Thm \ref{thm:LTI}) & Lipschitz-based & $\bar{x_1}$ & $\bar{x_2}$ & $\bar{x_3}$ & $\bar{x_4}$ \\
    \hline
      $u$ & 1.18164	& 0.02236	& 0.00166	& 0.01015 & 0.02522 & 0.24085 & 0.79849 \\
    $x_1$ & 0.21094	& 0.00186	& 0.00010	& 0.01012 & 0.02514 & 0.24011 & 0.79650\\
    $x_2$ & 0.13086	& 0.00205	& 0.00010	& 0.01027 & 0.02552 & 0.24368 & 0.80829\\
    $x_3$ & 1.33008	& 0.02227	& 0.00166	& 0.01012 & 0.02514 & 0.24009 & 0.79607 \\
    $x_4$ & 3.78516	& 0.05811	& 0.00439	& 0.01008 & 0.02504 & 0.23915 & 0.79299 \\
    \hline
    \end{tabular}%
    \end{adjustbox}
  \label{tab:add2}%
\end{table}%
